# Supplementary material for: Gradient Descent Ascent in Min-Max Stackelberg Games
Source: arXiv:2208.09690 source file (2022-08-20)
Supplement: Supplementary file 1 [file tables.tex]

\begin{table}[H]
    \centering
    \caption{Iteration complexities for min-max games with independent strategy sets in convex-concave settings. Note that these results assume that the objective function is Lipschitz-smooth.} \label{tab:fixed-convex-concave}
    \begin{tabular}{|c|c|c|}\hline
    Setting & Reference & Iteration Complexity \\ \hline
    \multirow{8}{*}{ $\mu_\outer$-Strongly-Convex- $\mu_\inner$-Strongly-Concave} & \cite{tseng1995variational} & \multirow{4}{*}{$\tilde{O}\left( \mu_\outer + \mu_\inner\right)$} \\\cline{2-2}
         & \cite{nesterov2006variational}  & \\ \cline{2-2}
         & \cite{gidel2020variational}     & \\ \cline{2-2}
         & \cite{mokhtari2020convergence}  &  \\ \cline{2-3}
         & \cite{alkousa2020accelerated}   & \shortstack{$\tilde{O}(\min \left\{\mu_\outer \sqrt{\mu_\inner}, \mu_\inner \sqrt{\mu_\outer}  ) \right\}$}\\ \cline{2-3}
         & \cite{lin2020near}              & $\tilde{O}(\sqrt{\mu_\outer \mu_\inner})$ \\ \cline{2-3}
         & \cite{ibrahim2019lower} & $\tilde{\Omega}(\sqrt{\mu_\outer \mu_\inner})$\\ \cline{2-2}
         & \cite{zhang2020lower} & \\ \hline \hline
    \multirow{3}{*}{$\mu_\outer$-Strongly-Convex-Linear}    & \cite{juditsky2011first} & \multirow{3}{*}{$O\left( \sqrt{\nicefrac{\mu_\outer}{\varepsilon}}\right)$} \\\cline{2-2}
    & \cite{hamedani2018primal} & \\\cline{2-2}
    & \cite{zhao2019optimal}& \\\hline \hline
    \multirow{3}{*}{$\mu_\outer$-Strongly-Convex-Concave} & \cite{thekumparampil2019efficient} & $\tilde{O}\left( \nicefrac{\mu_\outer }{\sqrt{\varepsilon}} \right)$ \\ \cline{2-3}
    & \cite{lin2020near} & $\tilde{O}(\sqrt{\nicefrac{\mu_\outer}{\varepsilon}})$ \\ \cline{2-3}
    & \cite{ouyang2018lower} & $\tilde{\Omega}\left( \sqrt{\nicefrac{\mu_\outer}{\varepsilon}}\right)$ \\ \hline \hline
    \multirow{5}{*}{Convex-Concave} & \cite{nemirovski2004prox} & \multirow{2}{*}{$O\left( \varepsilon^{-1}\right)$} \\ \cline{2-2}
    & \cite{nesterov2007dual} & \\ \cline{2-2}
    & \cite{tseng2008accelerated} & \\ \cline{2-3}
    & \cite{lin2020near} &  $\tilde{O}\left(\varepsilon^{-1}\right)$\\ \cline{2-3}
    & \cite{ouyang2018lower} & $\Omega(\varepsilon^{-1})$ \\ \hline 
    \end{tabular}
    
\end{table}

\begin{table}[H]
    \centering
    \caption{Iteration complexities for min-max games with independent strategy sets in non-convex-concave settings. Note that although all these results assume that the objective function is Lipschitz-smooth, some authors make additional assumptions: e.g., \cite{nouiehed2019solving} obtain their result for objective functions that satisfy the Lojasiwicz condition.}
    \label{tab:fixed-nonconvex-concave}
    
    \begin{tabular}{|c|c|c|}\hline
    Setting & Reference & Iteration Complexity\\ \hline
        \multirow{5}{*}{ \makecell{Nonconvex-$\mu_\inner$-Strongly-Concave,\\ First Order Nash  \\ or Local Stackelberg\\ Equilibrium}} & \cite{jin2020local} & \multirow{4}{*}{$ \tilde{O}(\mu_\inner^2 \varepsilon^{-2})$} \\
         & \cite{rafique2019nonconvex} & \\ \cline{2-2}
         & \cite{lin2020gradient}  & \\ \cline{2-2}
         & \cite{lu2019block} & \\ \cline{2-3}
         & \cite{lin2020near} & $\tilde{O}\left( \sqrt{\mu_\inner} \varepsilon^{-2} \right)$\\ \hline \hline
        \multirow{4}{*}{ \makecell{Nonconvex-Concave,\\ First Order \\ Nash Equilibrium}} & \cite{lu2019block}  & $\tilde{O}\left(\varepsilon^{-4}\right)$ \\ \cline{2-3}
        & \cite{nouiehed2019solving} & $\tilde{O}\left( \varepsilon^{-3.5}\right)$ \\ \cline{2-3}
        & \cite{ostrovskii2020efficient} & \multirow{2}{*}{$\tilde{O}\left( \varepsilon^{-2.5}\right)$} \\ \cline{2-2}
        & \cite{lin2020near} &  \\ \hline \hline
        \multirow{6}{*}{  \makecell{Nonconvex-Concave,\\ Local Stackelberg\\ Equilibrium}} & \cite{jin2020local} & \multirow{3}{*}{$\tilde{O}(\varepsilon^{-6})$}\\  \cline{2-2}
        & \cite{nouiehed2019solving} & \\ \cline{2-2}
        & \cite{lin2020near} & \\ \cline{2-3}
        & \cite{thekumparampil2019efficient} & \multirow{3}{*}{$\tilde{O}(\varepsilon^{-3})$}\\ \cline{2-2}
        & \cite{zhao2020prim} & \\
        & \cite{lin2020near} & \\ \hline 
    \end{tabular}
    
\end{table}
