# Supplementary material for: Gradient Descent Ascent in Min-Max Stackelberg Games
Source: arXiv:2208.09690 source file (2022-08-20)
Supplement: Supplementary file 2 [file algos.tex]

\section{Algorithm Pseudo-codes}\label{sec-app:algos}
