# Supplementary material for: Gradient Descent Ascent in Min-Max Stackelberg Games
Source: arXiv:2208.09690 source file (2022-08-20)
Supplement: Supplementary file 6 [file related.tex]

\section{Additional Related Work}\label{sec-app:related}

Much progress has been made recently in solving min-max games with independent strategy sets, both in the convex-concave case and in non-convex-concave case. We provide a survey of the literature as presented by \citeauthor{goktas2021minmax} in what follows.  
For the former case, when $\obj$ is $\mu_\outer$-strongly-convex in $\outer$ and $\mu_\inner$-strongly-concave in $\inner$, \citeauthor{tseng1995variational} \cite{tseng1995variational}, \citeauthor{nesterov2006variational} \cite{nesterov2006variational}, and \citeauthor{gidel2020variational} \cite{gidel2020variational} proposed variational inequality methods, and \citeauthor{mokhtari2020convergence} \cite{mokhtari2020convergence}, gradient-descent-ascent (GDA)-based methods, all of which compute a solution in $\tilde{O}(\mu_\inner + \mu_\outer)$ iterations.
These upper bounds were recently complemented by the lower bound of $\tilde{\Omega}(\sqrt{\mu_\inner \mu_\outer})$, shown by \citeauthor{ibrahim2019lower}  \cite{ibrahim2019lower} and  \citeauthor{zhang2020lower}   \cite{zhang2020lower}.
Subsequently, \citeauthor{lin2020near}  \cite{lin2020near} and   \citeauthor{alkousa2020accelerated} \cite{alkousa2020accelerated} analyzed algorithms that converge in $\tilde{O}(\sqrt{\mu_\inner \mu_\outer})$ and $\tilde{O}(\min\left\{\mu_\outer \sqrt{\mu_\inner}, \mu_\inner \sqrt{\mu_\outer} \right\})$ iterations, respectively. 

For the special case where $\obj$ is $\mu_\outer$-strongly convex in $\outer$ and linear in $\inner$, \citeauthor{juditsky2011first}  \cite{juditsky2011first},  \citeauthor{hamedani2018primal}  \cite{hamedani2018primal}, and \citeauthor{zhao2019optimal}  \cite{zhao2019optimal} all present methods that converge to an $\varepsilon$-approximate solution in $O(\sqrt{\nicefrac{\mu_\outer}{\varepsilon}})$ iterations.
When the strong concavity or linearity assumptions of $\obj$ on $\inner$ are dropped, and
$\obj$ is assumed to be $\mu_\outer$-strongly-convex in $\outer$ but only concave in $\inner$, \citeauthor{thekumparampil2019efficient} \cite{thekumparampil2019efficient} provide an algorithm that converges to an $\varepsilon$-approximate solution in $\tilde{O}(\nicefrac{\mu_\outer}{\varepsilon})$ iterations, and \citeauthor{ouyang2018lower} \cite{ouyang2018lower} provide a lower bound of $\tilde{\Omega}\left(\sqrt{\nicefrac{\mu_\outer}{\varepsilon}}\right)$ iterations on this same computation.
\citeauthor{lin2020near} then went on to develop a faster algorithm, with iteration complexity of $\tilde{O}\left(\sqrt{\nicefrac{\mu_\outer}{\varepsilon}}\right)$, under the same conditions.

When $\obj$ is simply assumed to be convex-concave, \citeauthor{nemirovski2004prox} \cite{nemirovski2004prox}, \citeauthor{nesterov2007dual} \cite{nesterov2007dual}, and \citeauthor{tseng2008accelerated} \cite{tseng2008accelerated} describe algorithms that solve for an $\varepsilon$-approximate solution with $\tilde{O}\left(\varepsilon^{-1}\right)$ iteration complexity, and \citeauthor{ouyang2018lower} \cite{ouyang2018lower} prove a corresponding lower bound of $\Omega(\varepsilon^{-1})$.

When $\obj$ is assumed to be non-convex-$\mu_\inner$-strongly-concave, and the goal is to compute a first-order Nash, \citeauthor{sanjabi2018stoch} \cite{sanjabi2018stoch} provide an algorithm that converges to $\varepsilon$-an approximate solution in $O(\varepsilon^{-2})$ iterations.
\citeauthor{jin2020local} \cite{jin2020local}, \citeauthor{rafique2019nonconvex} \cite{rafique2019nonconvex}, \citeauthor{lin2020gradient} \cite{lin2020gradient}, and \citeauthor{lu2019block} \cite{lu2019block} provide algorithms that converge in $\tilde{O}\left(\mu_\inner^2 \varepsilon^{-2}\right)$ iterations, while \citeauthor{lin2020near} \cite{lin2020near} provide an even faster algorithm, with an iteration complexity of $\tilde{O}\left(\sqrt{\mu_\inner} \varepsilon^{-2}\right)$.

%\deni{We use the word local for Stackelberg and that definition is indeed a local definition, but first-order Nash is not really local, it is a bit weirder than that, i.e., it is a Nash eqm in which players cannot make improvement in utility by only making deviations based on first order information *about the objective function*.} \amy{we have local minimax in the last paragraph of the conclusion.} \deni{Local minimax is actually local Stackelberg!!! A minimax point is what Jordan calls Stackelberg equilibria and then Dai et al. introduce a local version of minimax, which is essentially local Stackelberg! So for them when you say a minimax point they just mean a solution to the min-max problem but not necessarily to the max-min problem. Note that their definition is different than Costis' where costs defines a minimax point as a saddle point}.
%\denit{A first-order Nash is a stationary point of the objective function for both players, while a local Stackelberg eqm is a point for which the value function's gradient is 0 for the min player and the gradient of the objective is 0 for the max player. The difference between the two are basically simultaneous game vs. sequential game.}

When $\obj$ is non-convex-non-concave and the goal to compute is an approximate first-order Nash equilibrium, \citeauthor{lu2019block} \cite{lu2019block} provide an algorithm with iteration complexity $\tilde{O}(\varepsilon^{-4})$, while \citeauthor{nouiehed2019solving} \cite{nouiehed2019solving} provide an algorithm with iteration complexity $\tilde{O}(\varepsilon^{-3.5})$. More recently, \citeauthor{ostrovskii2020efficient} \cite{ostrovskii2020efficient} and \citeauthor{lin2020near} \cite{lin2020near} proposed an algorithm with iteration complexity $\tilde{O}\left(\varepsilon^{-2.5}\right)$.

When $\obj$ is non-convex-non-concave and the desired solution concept is a ``local'' Stackelberg equilibrium, \citeauthor{jin2020local} \cite{jin2020local}, \citeauthor{rafique2019nonconvex} \cite{rafique2019nonconvex}, and \citeauthor{lin2020gradient} \cite{lin2020gradient} provide algorithms with a $\tilde{O}\left( \varepsilon^{-6} \right)$ complexity.
More recently, \citeauthor{thekumparampil2019efficient} \cite{thekumparampil2019efficient}, \citeauthor{zhao2020prim} \cite{zhao2020prim}, and \citeauthor{lin2020near} \cite{lin2020near} have proposed algorithms that converge to an $\varepsilon$-approximate solution in $\tilde{O}\left( \varepsilon^{-3}\right)$ iterations.

We summarize the literature pertaining to the convex-concave and the non-convex-concave settings in Tables 1 and 2
% Tables~\ref{tab:fixed-convex-concave} and~\ref{tab:fixed-nonconvex-concave}, 
respectively.
